# Supplementary material for: VeriSolid: Correct-by-Design Smart Contracts for Ethereum
Source: arXiv:1901.01292 source file (2019-01-21)
Supplement: Supplementary file 1 [file appendix.tex]

\section{Simple Deadlocked Contract}

\begin{figure} [t]
\centering
\includegraphics[scale=1]{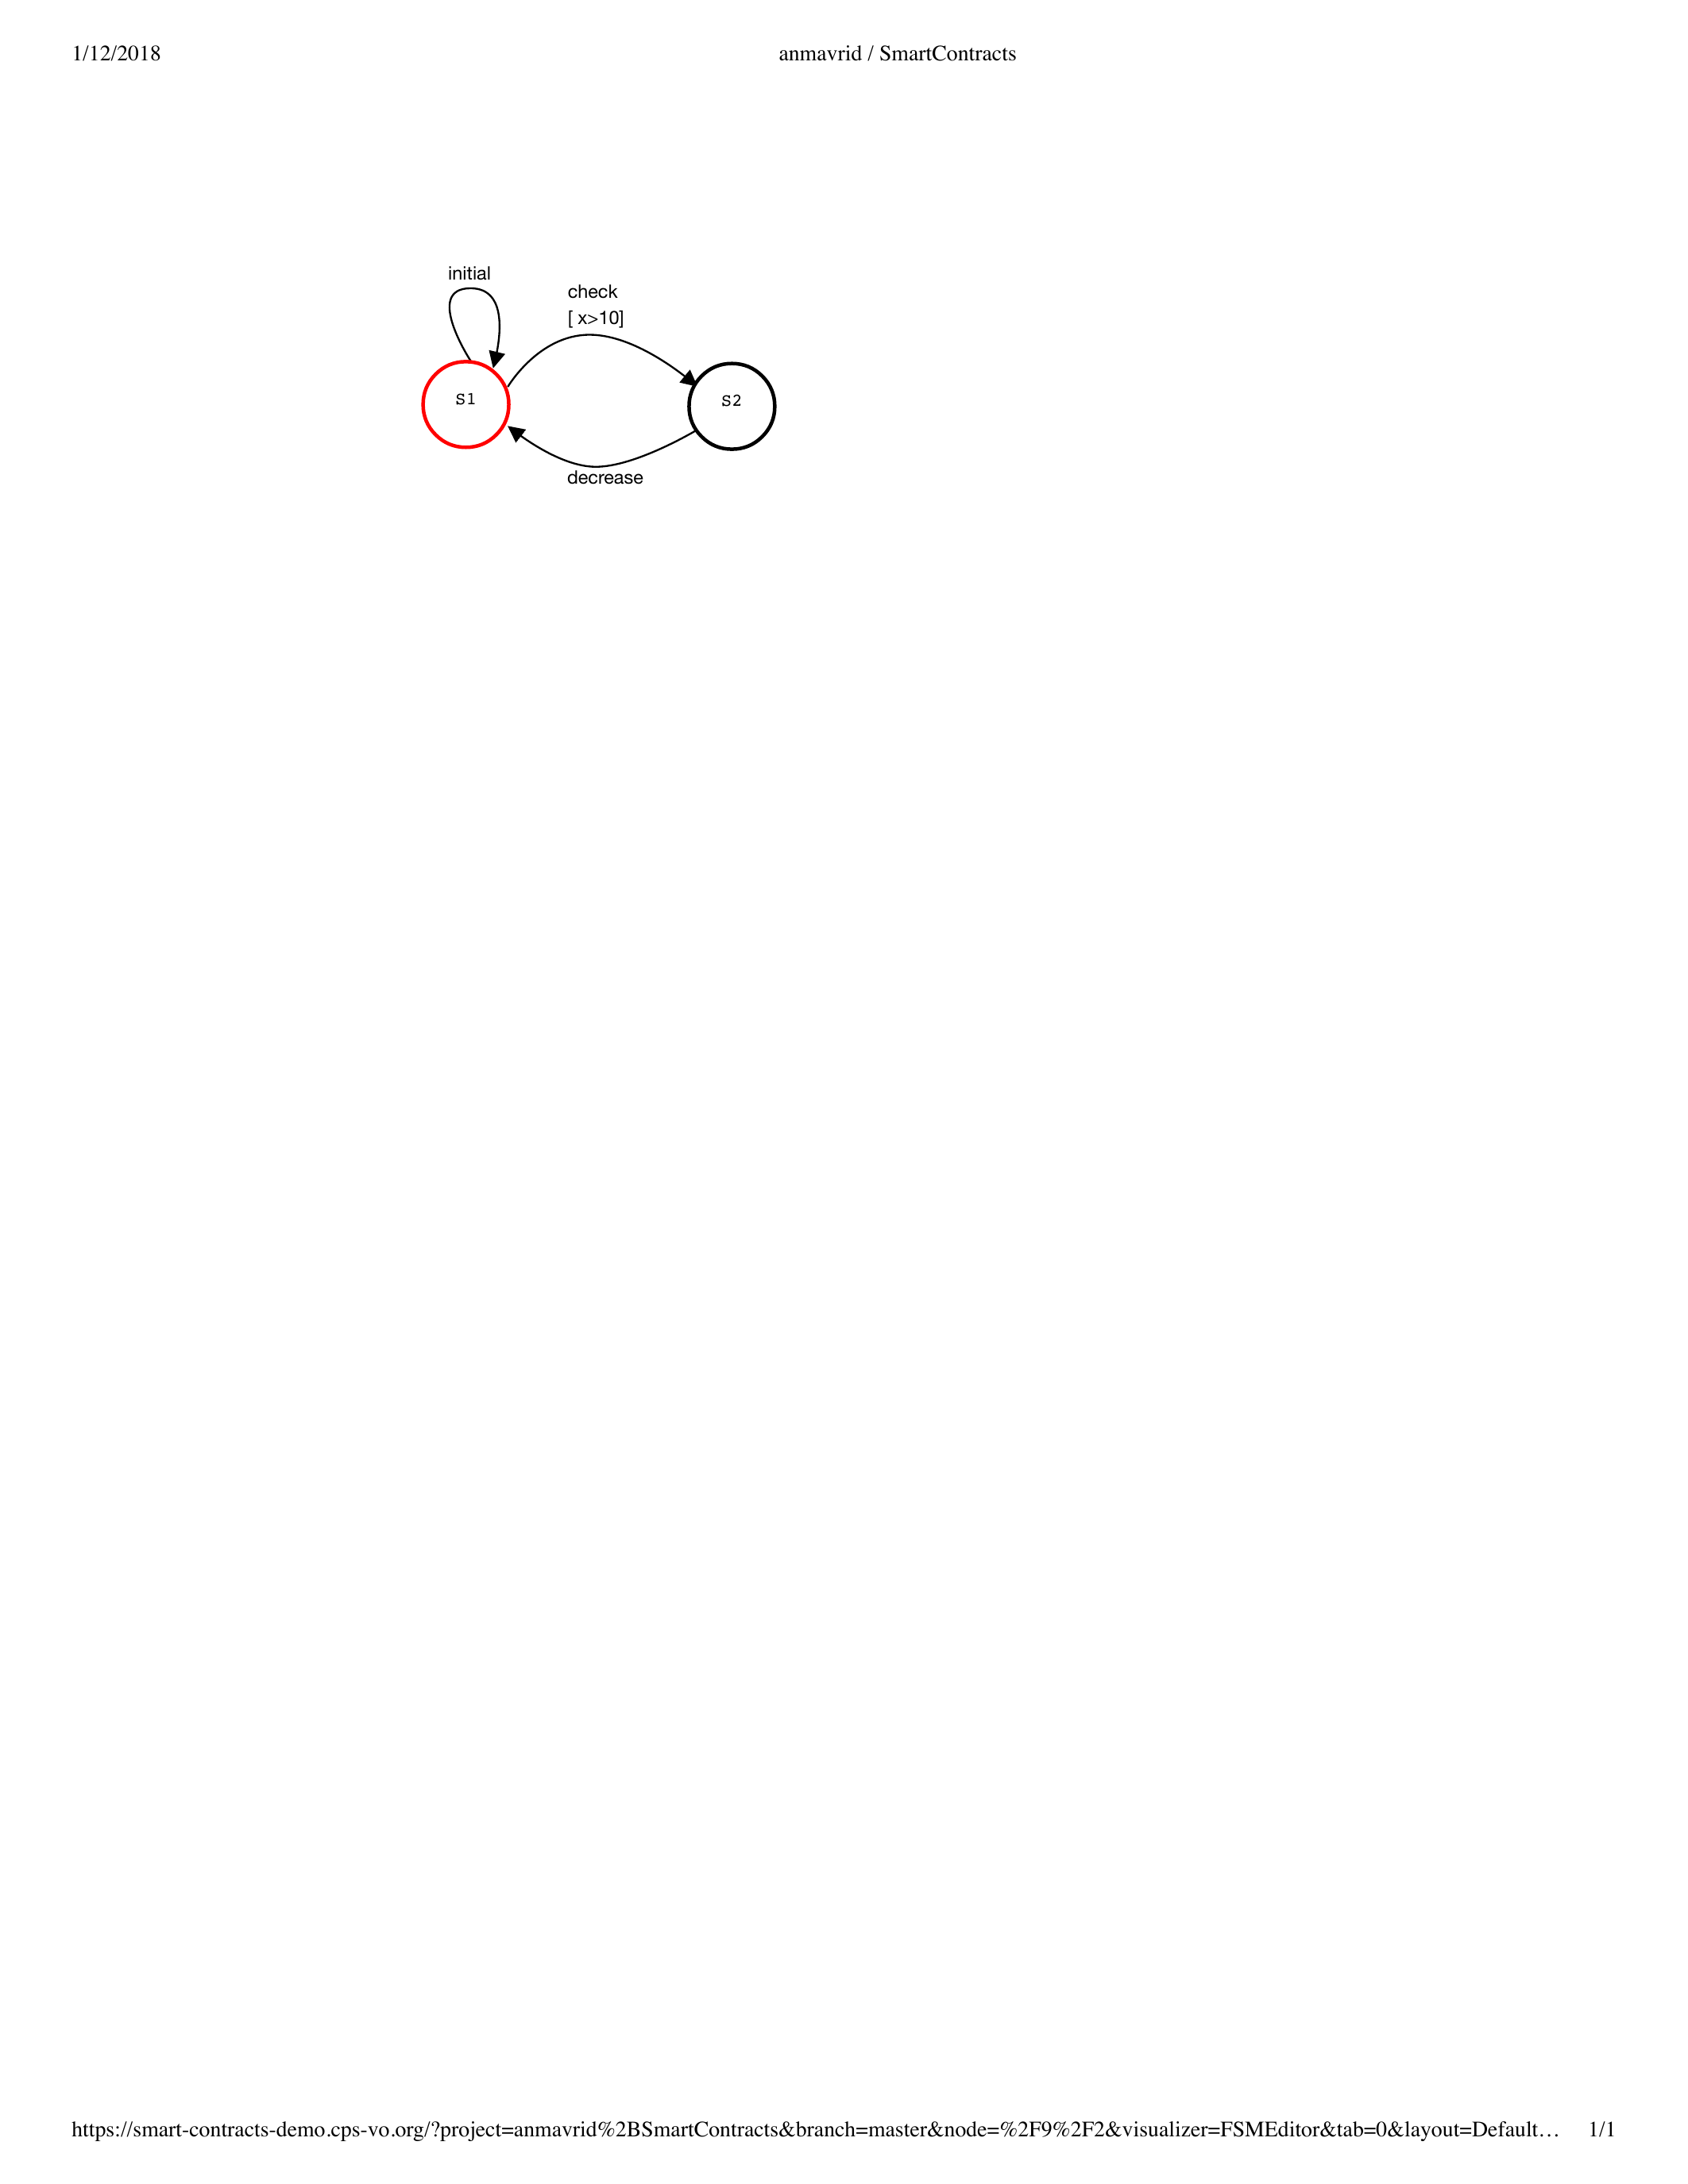}
\caption{Simple Deadlocked Contract.}
\label{fig:blauction}
\end{figure}

\begin{lstlisting} [style=customjava]
contract SimpleContract {
  uint private creationTime = now;
  //States definition
  enum States {
    S1, 
    S2 
  }
  States private state = States.S1;
  //Insert variable definitions

  //Transitions 
  function check () public 
  {
  	require(state == States.S1);
  	//Guards
  	require(x>10);     
  	//State change
  	state = States.S2; 
  }

  function decrease () public 
  {
      require(state == States.S2);
      //Actions
      x=x-1;   
      //State change
      state = States.S1; 
  }

  function initial () public 
  {
      require(state == States.S1);
      //Actions
      x = 10;   
  }
}
\end{lstlisting}

\begin{lstlisting} [style=custombip]
package SimpleContract
	port type portType()
	atom type SimpleFSM()
 		data int x

 		place S1, S2
 
 		initial to S1 do { x=10; }

 		on t1 from S1 to S2 provided (x > 0)
 		on t2  from S2 to S1 do {x=x-1;}
	end
end
\end{lstlisting}

\section{Solidity code}
\begin{lstlisting}[style=customjava]
contract BlindAuction{
    //States definition
    enum States {
        ABB,
        RB,
        F,
        C
    }
    States private state = States.ABB;
    
    //Variables definition
    struct Bid {
        bytes32 blindedBid;
        uint deposit;
    }
    mapping(address => Bid[]) private bids;
    mapping(address => uint) private pendingReturns;
    address private highestBidder;
    uint private highestBid;
    uint private creationTime = now;
    
    //Transitions
    //Transition bid
    function bid (bytes32 blindedBid)
        payable
    {
        require(state == States.ABB);
        //Actions
        bids[msg.sender].push(Bid({
            blindedBid: blindedBid,
            deposit: msg.value
        }));
        pendingReturns[msg.sender] += msg.value;
    }
    
    //Transition close
    function close()
    {
        require(state == States.ABB);
        //Guards
        require(now >= creationTime + 5 days);
        //State change
        state = States.RB;
    }
    
    //Transition reveal
    function reveal(uint[] values, bytes32[] secrets)
    {
        require(state == States.RB);
        //Guards
        require(values.length == secrets.length);
        //Actions
        for (uint i = 0; i < values.length && 
                i < bids[msg.sender].length; i++) {
            var bid = bids[msg.sender][i];
            var (value, secret) = (values[i], secrets[i]);
            if (bid.blindedBid != keccak256(value, secret)) {
                // Do not add to refund value.
                continue;
            }
            if (bid.deposit >= value && value > highestBid) {
                    highestBid = value;
                    highestBidder = msg.sender;
            }
        }
    }
    
    //Transition finish
    function finish()
    {
        require(state == States.RB);
        //Guards
        require(now >= creationTime + 10 days);
        //State change
        state = States.F;
    }
    
    //Transition cancel
    function cancelABB()
    {
        require(state == States.ABB);
        //State change
        state = States.C;
    }
    
    //Transition cancel
    function cancelRB()
    {
        require(state == States.RB);
        //State change
        state = States.C;
    }
    
    //Transition withdraw
    function withdraw()
    { 
        uint amount;
        require(state == States.F);
        //Actions
        amount = pendingReturns[msg.sender];
        if (amount > 0 && msg.sender!= highestBidder) {
            msg.sender.transfer(amount); // REENTRANCY VULNERABILITY
            pendingReturns[msg.sender] = 0;
        } else {
            msg.sender.transfer(amount - highestBid); // REENTRANCY VULN.
            pendingReturns[msg.sender] = 0;
        }
    }
    
    //Transition unbid
    function unbid()
    {
        uint amount;
        require(state == States.C);
        //Actions
        amount = pendingReturns[msg.sender];
        if (amount > 0) {
            msg.sender.transfer(amount); // REENTRANCY VULNERABILITY
            pendingReturns[msg.sender] = 0;
        }
    }   
}
\end{lstlisting}
